# Supplementary material for: Dynamics of Protein Hydration Water
Source: arXiv:1412.2698 source file (2014-12-08)
Supplement: Supplementary file 1 [file Wolf-Supplemental_Material.pdf]

# Dynamics of Protein Hydration Water

## Supplemental Material

Martin Wolf,* S. Emmert, R. Gulich, P. Lunkenheimer, and A. Loidl
*Experimental Physics V, Center for Electronic Correlations and Magnetism, University of Augsburg, Universitätsstr. 2, 86135 Augsburg, Germany*

### Materials and methods

The complex dielectric permittivity and conductivity were determined using two different measurement devices [1, 2] to cover the most interesting frequency range of about 0.1 Hz–3 GHz. For the low-frequency range (0.1 Hz–10 MHz) a Novocontrol Alpha-A Analyzer was employed. This frequency-response analyzer enables high precision measurements by directly measuring the sample voltage and the sample current by means of a lock-in technique. The sample is kept in a parallel-plate capacitor made of platinum (diameter 4.8 mm, plate distances $d$ =0.1–0.85 mm), which is mounted into a $N_2$-gas cryostat (Novocontrol Quatro) allowing for temperature-dependent measurements. In the frequency range 1 MHz–3 GHz, a coaxial reflection method was used employing the Agilent Impedance/Material Analyzer E4991A. Here, the sample capacitor is connected to the end of a coaxial line, thereby bridging inner and outer conductor. To eliminate contributions of coaxial line and connectors, a calibration with three standard impedances is necessary. Temperature-dependent measurements are enabled by placing the capacitor in a $N_2$-gas cryostat (Novocontrol Quatro). The connection between sample and the measurement device within the cryostat is established by a specially designed sample holder [1].

Dialyzed and lyophilized hen egg white lysozyme powder ($M$ = 14.3 kDa) was purchased from Sigma-Aldrich (Fluka 62970) and used without further purification. Lysozyme/water solutions (mixtures) were prepared by dissolving weighed amounts of protein powder in deionized $H_2O$ (Merck "Ultrapur"). In this way, protein solutions with concentrations between 3 mmol and 100 mmol of protein per liter of water were prepared (corresponding to 42.9 mg–1430 mg of protein per ml of water, room temperature). The pH values of these solutions are in the range 2.8–3.8 (measured with a pH tester from Hanna-Instruments). The hydrated lysozyme powder was prepared by exposing the powder of the same type as above (Fluka 62970) to an atmosphere with a defined relative humidity of $rH$ = 97–98 % ($T$ = 25 °C), ensured by a saturated $K_2SO_4$ solution in an exsiccator. The degree of hydration was determined to be $h$ = 30 wt%, i.e. 0.3 g of water per gram of sample.

### Broadband complex permittivity of the 10 mmol/l lysozyme solution

Figure 1 shows the frequency dependence of the dielectric constant (as shown in Fig. 2(a) of the main article) and the corresponding dielectric loss. As mentioned in the article, there are three relaxations besides the two $\delta$-relaxations. Except for the strongest relaxation (EP1), the corresponding relaxation peaks of the dielectric loss are superimposed by the strong dc conductivity contributing to the dielectric loss according to $\varepsilon''(\nu) = \sigma'/(\varepsilon_0 2\pi\nu)$, which gives rise to a $1/\nu$ divergence in $\varepsilon''(\nu)$ for decreasing frequencies. With decreasing temperature, the ice relaxation emerges and can clearly be seen for the lowest temperature shown (180 K). The solid lines are fits using the sum of five Cole-Cole functions to account for the five relaxations found.

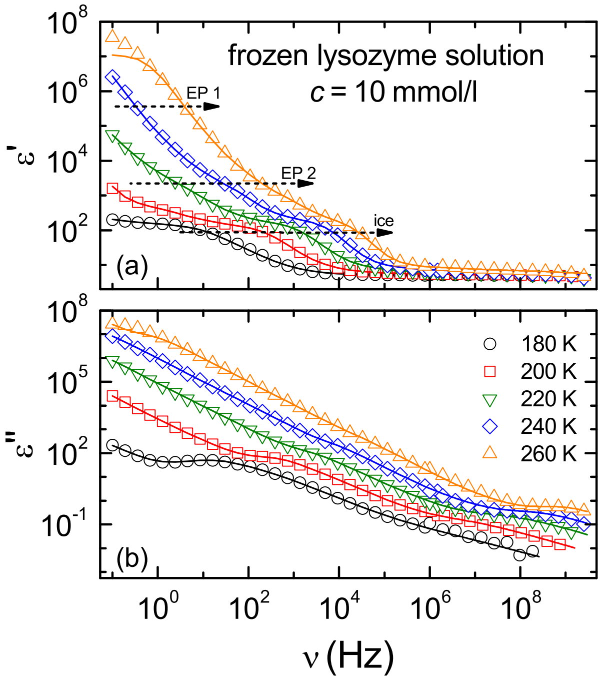


FIG. 1. Dielectric constant (a) and dielectric loss (b) of a 10 mmol/l lysozyme solution measured at different temperatures below 273 K. Solid lines are fits using the sum of five Cole-Cole functions.

### First derivative of the dielectric loss and significance of the fragile-to-strong transition

Figure 2 shows the high-frequency part of (a) the dielectric loss $\varepsilon''(\nu)$ of the 5 mmol/l lysozyme solution and (b) the derivative $\partial \log(\varepsilon'')/\partial \log(\nu)$ (= slope), in the temperature range 180–270 K. As mentioned in the main article, the significance of the fragile-to-strong transition found for the temperature dependence of the relaxation times at around 210 K is limited. This is due to the fact that the exact loss-peak positions are difficult to determine for the low-temperature curves (see Fig. 2(a)). Therefore, the slope of the curves was determined by calculating the first derivative of the dielectric loss (b). The maxima in (b) correspond to the points with the most shallow slope in the experimental data, indicating a step in $\varepsilon''(\nu)$ caused by an underlying relaxation peak. In this way, the temperature dependence of the $\delta_2$-relaxation can be tracked. Starting at 270 K, the peak strongly shifts with decreasing temperature but then gets stuck somewhere below 210 K. This finding seems to support the fragile-to-strong transition of the relaxation times (Fig. 3 of the main article).

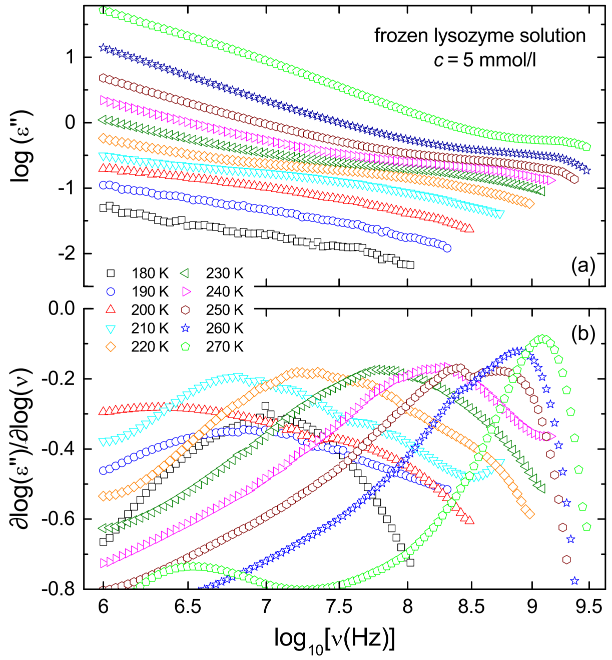


FIG. 2. (a) Frequency dependence of the dielectric loss of the 5 mmol/l lysozyme solution for temperatures below the freezing point. (b) First derivative $\partial \log(\varepsilon'')/\partial \log(\nu)$ of the data shown in (a). To avoid excessive scattering, before calculating the derivatives, the data in (a) were smoothed by Savitzky–Golay filtering using 5th-order polynomials.

* Corresponding author. Martin.Wolf@physik.uni-augsburg.de

[1] R. Böhmer, M. Maglione, P. Lunkenheimer, and A. Loidl, J. Appl. Phys. **65**, 901 (1989).

[2] U. Schneider, P. Lunkenheimer, A. Pimenov, R. Brand, and A. Loidl, Ferroelectrics **249**, 89 (2001).
